# Supplementary material for: Controllable Length Control Neural Encoder-Decoder via Reinforcement Learning
Source: arXiv:1909.09492 source file (2019-09-17)
Supplement: Supplementary file 1 [file ss_appendix.tex]

\clearpage
\begin{appendices}

%--------------------------------*--------------------------------%
%------------------------*------* *------*------------------------%
%-----------------------* *----*   *----* *-----------------------%
%----------------------* E *--*  Y  *--* E *----------------------%
%-----------------------* *----*   *----* *-----------------------%
%------------------------*------* *------*------------------------%
%--------------------------------*--------------------------------%

    \section{Formulation}

    \begin{itemize}
        \item $\mathcal{D}$: dataset
        \item $\mathbf{x} = \{ x_1, x_2, \dotsb, x_N \}$ : nput tokens
        \item $\mathbf{y} = \{ y_1, y_2, \dotsb, y_M \}$ : predicted output tokens
        \item $\mathbf{y}^* = \{ y_1^*, y_2^*, \dotsb, y_M^* \}$ : ground truth output tokens
        \item $\mathbf{y}^s = \{ y_1^s, y_2^s, \dotsb, y_M^s \}$ : multinomial sampled tokens
        \item $y_{1:t}$ = $\{ y_1, y_1,\dots, y_t \} $
        \item $\parallel$ : concate operation
        \item $\otimes$: matrix productino
        \item $h_i^d$ : hidden state for $i^{th}$ decoder LSTM
        \item $m_i^d$ : memory cell for $i^{th}$ decoder LSTM
        \item $h_i^e$ : hidden state for $i^{th}$ encoder LSTM
        \item $m_i^e$ : memory cell for $i^{th}$ encoder LSTM
    \end{itemize}

    \subsection{Seq2Seq Model}

    The training objective is to maximize the log likelihood of the sentence-summary paris
    of dataset $\mathcal{D}$:
    \begin{align}
        L_{ml}(\theta) = \sum_{\mathbf{x}, \mathbf{y} \in \mathcal{D}} \log p(\mathbf{y}|\mathbf{x}; \theta)
    \end{align}

    The problem can be formulated as conditional probability
    \begin{align}
        p(\mathbf{y}|\mathbf{x}; \theta) = \prod_{t=1}^m p(y_t|y_{1:t-1}, \mathbf{x})
    \end{align}

    every time we caculate the probability distribution of generating the next word
    from current hidden state and attention vector

    \begin{align}
        p(y_{t}|y_{1:t-1}, \mathbf{x}) = \mathop{softmax}\left( W(h_t^d \parallel c_t) + b \right)
    \end{align}

    The whole model using seq2seq structure, LSTM is adopted for encoder and decoder
    our model using bi-directional LSTM encoder to generate hidden state in each time step:
    \begin{align}
        h_t^e = f_{LSTM}^{enc}(h_{t-1}^e, x_t) \\
        h_t^d = f_{LSTM}^{dec}(h_{t-1}^d, y_t)
    \end{align}

    We also adopt attention machenism for our model,
    \begin{align}
        e_{t,i} = v^T \tanh (W h_t^d + W h_i^e + b)
    \end{align}
    \begin{align}
        \alpha_{t,i} = \frac{\exp{e_{t,i}}}{\sum_{j=1}^N \exp(e_{t,j})}
    \end{align}
    \begin{align}
        c_t = \sum_{i=1}^N \alpha_{t,i} h_i^e
    \end{align}

    \subsection{Length Control}

    To control the length by neural encoder-decoder, there are two method proposed by yuta.

    lenmeb: desired length at each time for remaining sentence step embedding is treated as additional input with word embedding:
    \begin{align}
        h_t^d = f_{LSTM}^{dec}(h_{t-1}^d, m_{t-1}^d, y_t \parallel l_t)
    \end{align}

    leninit: desired length of the whole sentence is feed into init state of memory cell of decoder:
    \begin{align}
        m_0^d = b_l \otimes l_0
    \end{align} 
    $b_l$ is a trainable parameter.

    \subsection{Reinforcement Learning}
    LSTM Model can be viewed as an agent, the parameter of the network make a policy $p_{\theta}$, make prediction
    at each step can be view as action, Upon generating the end-of-sequence the agent receive a reward evaluate by 
    rouge metric. The reward is evaluated with ground truth summary, we denote this reward by $r$. 
    In reinforcement learning, the goal is to minimie the negative expected reward:
    \begin{align}
        L_{rl} (\theta) = - E_{y\sim p_{\theta}} [r(\mathbf{y})] 
    \end{align}
    To achieve the above objective, an intuitive idea is to enlarge the probability for which provide better score. 
    the gradient of the reward function is:
    \begin{align}
        \nabla_{\theta} L_{rl} (\theta) = - E_{y\sim p_{\theta}} [r(\mathbf{y})] \nabla_{\theta} \log p_{\theta} (\mathbf{y})
    \end{align} 
    
    The policy gradient given by reinforcement learning can be generalized to compute the reward 
    associated with an action value relative to a reference reward or baseline b,
    \begin{align}
        \nabla_{\theta} L_{rl} (\theta) = - E_{y\sim p_{\theta}} [r(\mathbf{y}) - b] \nabla_{\theta} \log p_{\theta} (\mathbf{y})
    \end{align} 
    the baseline b can be the evaluate score of greedy sample of the decoder. 
    \begin{align}
        \nabla_{\theta} L_{rl} (\theta) = - E_{y\sim p_{\theta}} [r(\mathbf{y}^s) - r(\mathbf{y})] \nabla_{\theta} \log p_{\theta} (\mathbf{y})
    \end{align}

    In practice the expected gradient can be approximated using a single Monte-Carlo sample
    \begin{align}
        \nabla_{\theta} L_{rl} (\theta) \approx \sum_i (r(\mathbf{y}^s_i) - r(\mathbf{y}_i)) \nabla_{\theta} \log p_{\theta} (\mathbf{y}_i)
    \end{align}
    One way to remedy this is to learn a policy that maximizes a specific discrete metric instead of 
    minimizing the maximum-likelihood loss, which is made possible with reinforcement learning.

    \subsection{Controlable length control by RL}
    
    to add a control unity to the model, we add a linear layer before enter the decoder as input.
    here, we propose two new model for reinforcement learning. 

    lenLinit: 
    \begin{align}
        m_0 = W(\bar{b}_{gauss} \otimes l_0) 
    \end{align}

    lenLemb:
    \begin{align}
        h_t^d = f_{LSTM}^{dec}(h_{t-1}^d, m_{t-1}^d + W(\bar{b}_{gauss} \otimes l_t)  , y_t)
    \end{align}

    The reward for the sentence is setted as the sum of rouge score:
    \begin{align}
        r(\mathbf{y}) = \text{rouge}_1(\mathbf{y}) + \text{rouge}_2(\mathbf{y}) + \text{rouge}_l(\mathbf{y})
    \end{align}
    To make the control ability in reinforcement learning process, the reward for final framework is:

    We specific the distance of the expected length and sampled sentence as:
    \begin{align}
        dis = \text{len}(\mathbf{y}^s) - l_0
    \end{align}
    then we select the reward by the dis we defined.
    \begin{equation}
        r(\mathbf{y}) =\left \{ \begin{array}{lll} r(\mathbf{y}) & condiaiton\ a \\ 0 & otherwise \end{array} \right.
    \end{equation}
    nonlinear is forbidden in our model, cause it will degrade the length information.
    
    the condition a here is that $dis < dis_{thres}$ and if the $dis$ exceed the $dis_thres$ then we define a 
    probability $p < 1.0$, random sample a number $p_s < 1.0$ and the condition is then become $p_s < p$.

\end{appendices}
